# Supplementary material for: Learning Self-Supervised Low-Rank Network for Single-Stage Weakly and Semi-Supervised Semantic Segmentation
Source: arXiv:2203.10278 source file (2022-03-19)

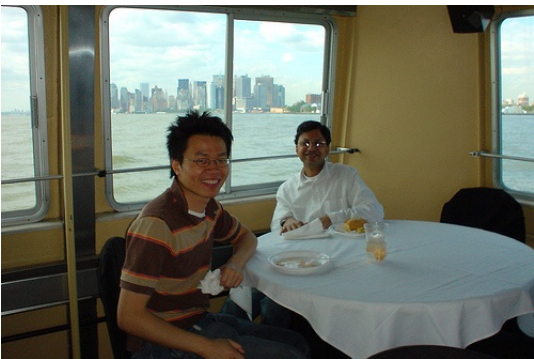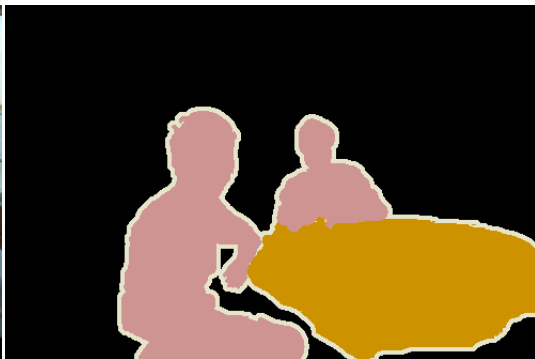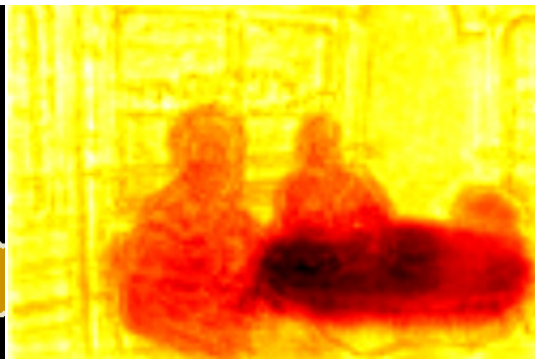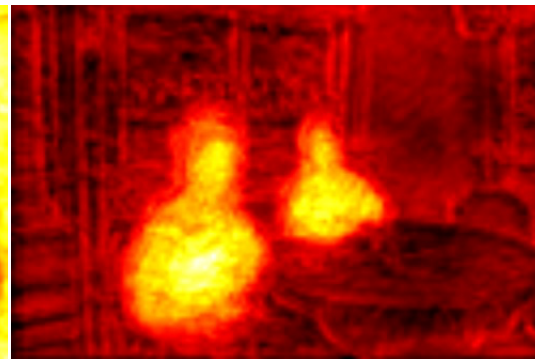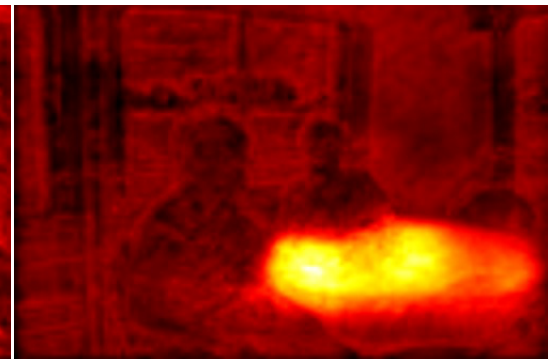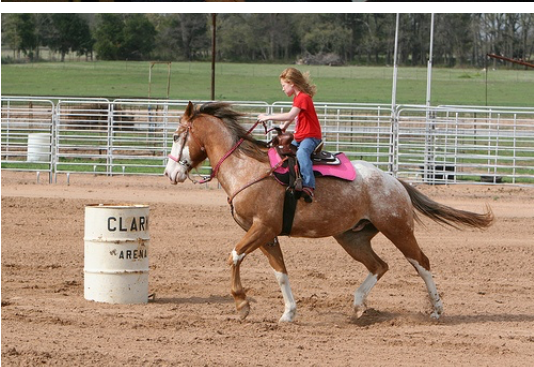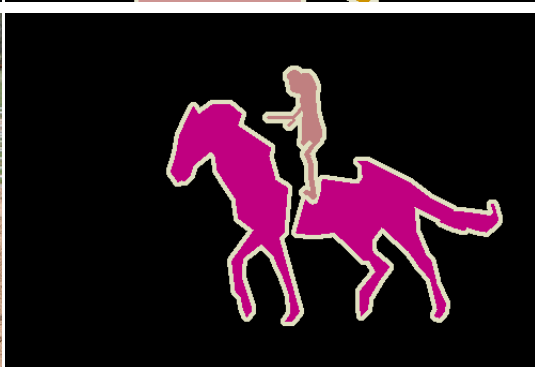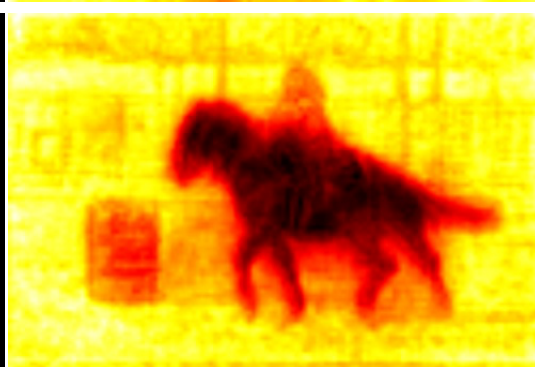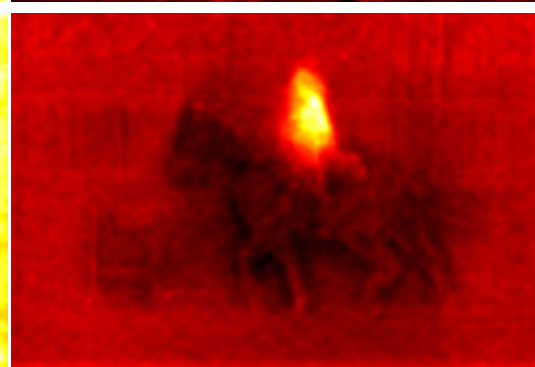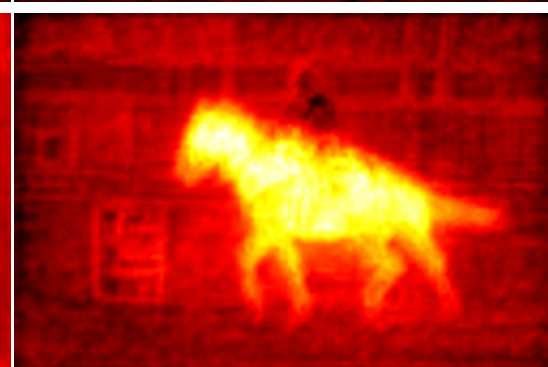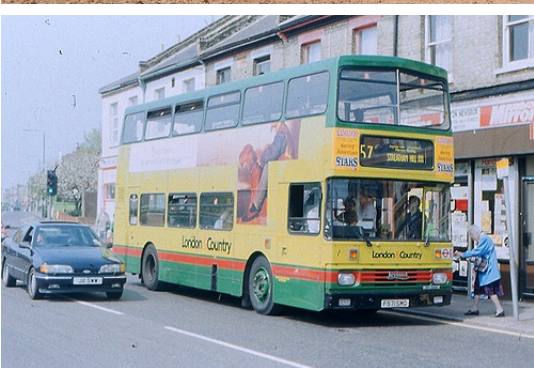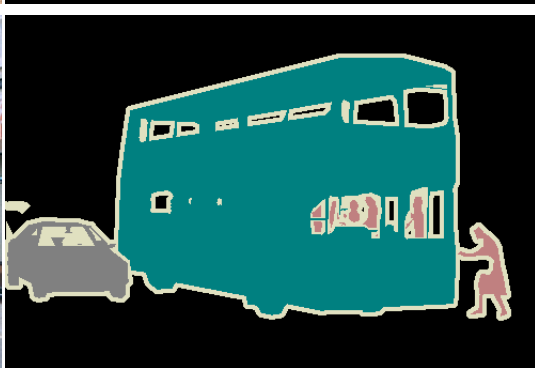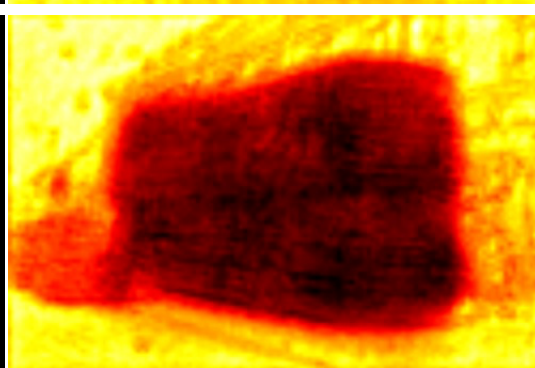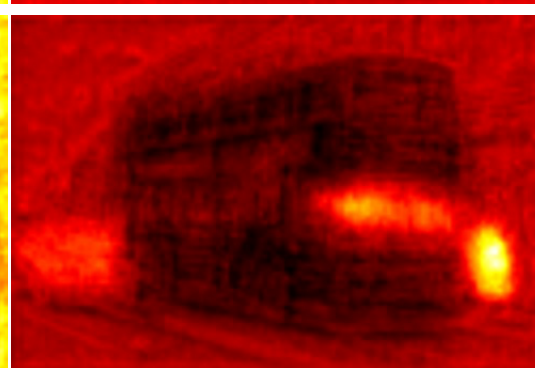

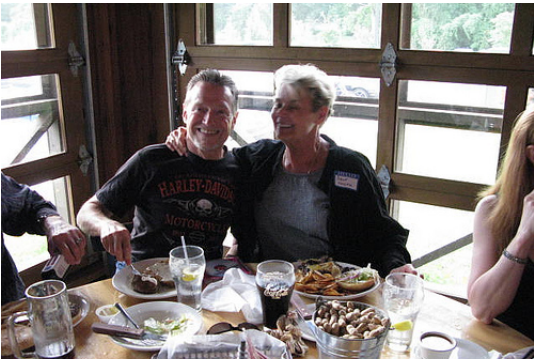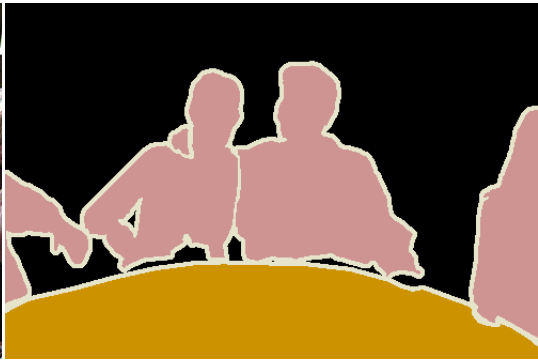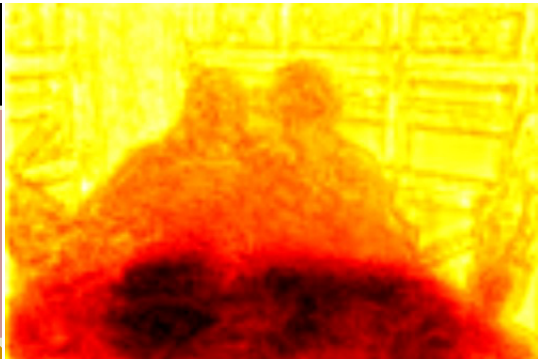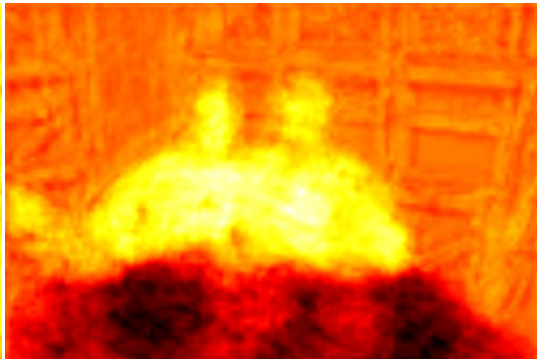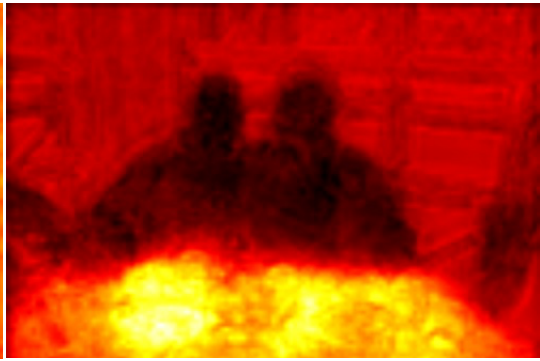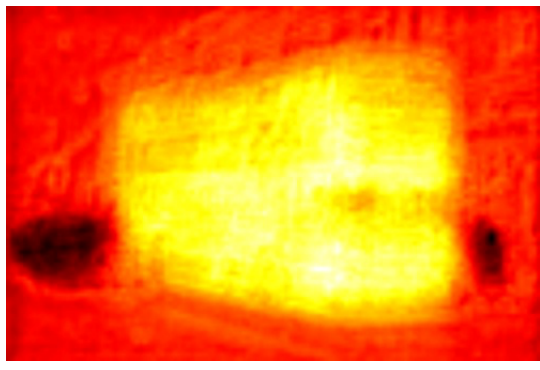

Supplement: Supplementary file 1 [file supp_assignments.pdf]
